# Supplementary material for: CrossModalQA: A Cross-modal and Multi-hop Benchmark for Multimodal Retrieval-augmented Generation
Source: arXiv:2609.05518 source file (2026-08-31)
Supplement: Supplementary file 1 [file 5-examples.tex]

% \section{Data Examples}
 
% Figure~\ref{fig:prompt123} and~\ref{fig:prompt45} illustrate examples of QA pairs from different modes in CrossModalQA.
